# Supplementary material for: ParTEETor: A System for Partial Deployments of TEEs within Tor
Source: arXiv:2408.14646 source file (2024-08-26)
Supplement: Supplementary file 1 [file appendix.tex]

\section{Attack Figures}\label{figs}
In this appendix, we provide figures depicting each class of attack analyzed in section~\ref{methodology1}.

%\shortsection{Replay Attack}
\begin{figure}[!h]
\centering
\centerline{\includegraphics[scale=0.5]{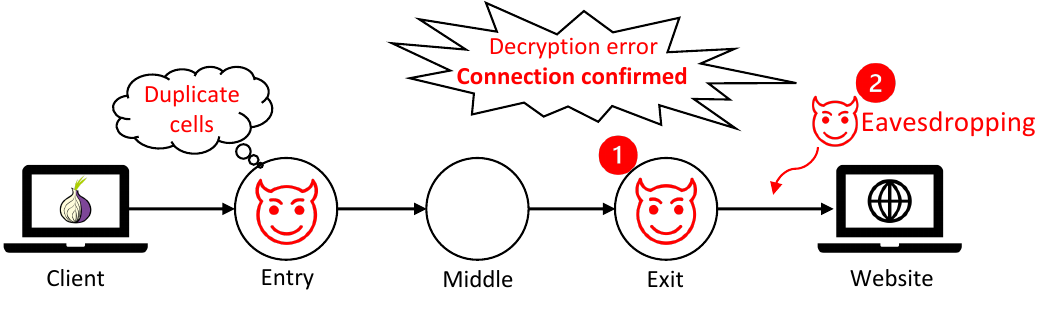}}
\caption{Replay Attack Scenario}
\label{fig:replay_attack}
\end{figure}

%\shortsection{Onion Services Attack}
\begin{figure}[!h]
\centering
\centerline{\includegraphics[scale=0.5]{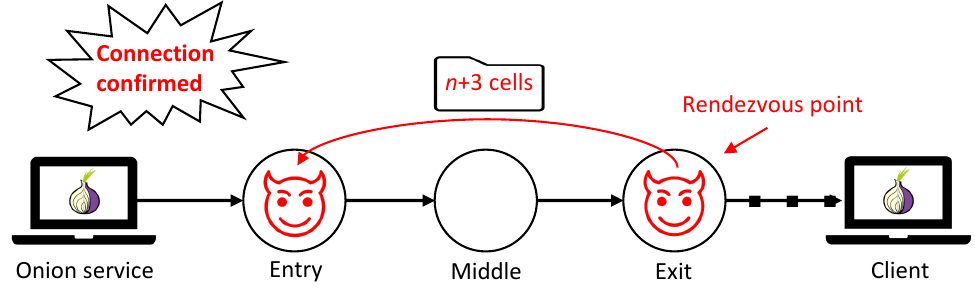}}
\caption{Onion Services Attack Scenario}
\label{fig:hidden_services_attack}
\end{figure}

%\shortsection{Fingerprinting Attack}
\begin{figure}[!h]
\centering
\centerline{\includegraphics[scale=0.5]{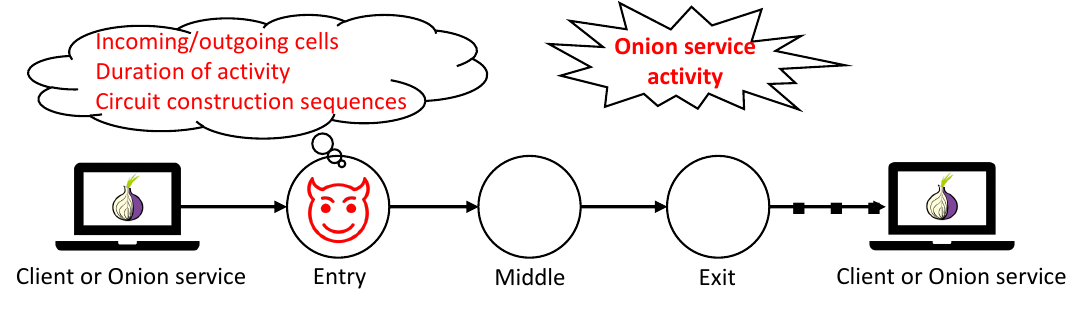}}
\caption{Fingerprinting Attack Scenario}
\label{fig:fp_attack}
\end{figure}

%\shortsection{Bad Apple Attack}
\begin{figure}[!h]
\centering
\centerline{\includegraphics[scale=0.5]{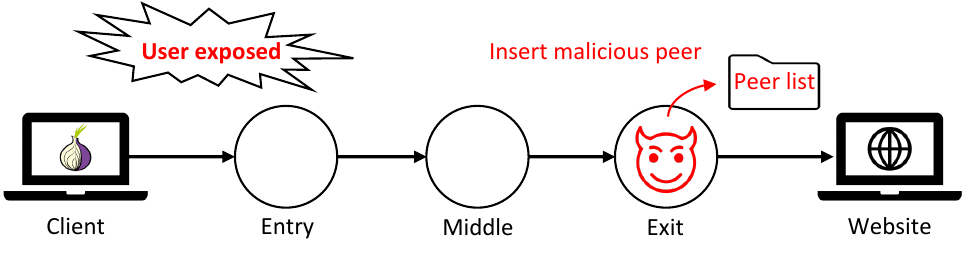}}
\caption{Bad Apple Attack Scenario}
\label{fig:bad_apple_attack}
\end{figure}

%\shortsection{Bandwidth Inflation Attack}
\begin{figure}[!h]
\centering
\centerline{\includegraphics[scale=0.5]{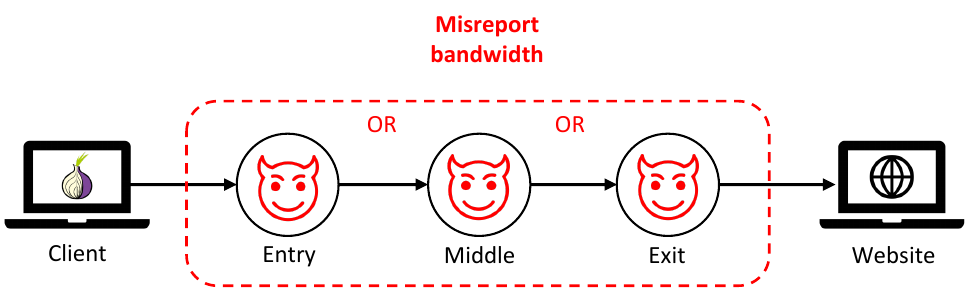}}
\caption{Bandwidth Inflation Scenario}
\label{fig:bandwidth_inflation}
\end{figure}
